# Supplementary material for: RealGen: Retrieval Augmented Generation for Controllable Traffic Scenarios
Source: arXiv:2312.13303 source file (2024-08-13)
Supplement: Supplementary file 1 [file X_suppl.tex]

\clearpage
\appendix
\setcounter{page}{1}

\section{Training and Model Details}
\label{sec:hyper_parameters}

\subsection{Details of model architecture}

In addition to the model architecture introduced in Algorithm~\ref{alg:encoder-decoder}, we also want to provide more details about the spatial-temporal transformer structure. For the projected embedding with shape $[B, M, T, H]$ with batch size $B$, we reshape it to shape $[T, B\times M, H]$ and treat $T$ as the sequence dimension. Then we add a positional embedding to it before putting it into the temporal transformer encoder. After that, we reshape it to $[M, B\times T, H]$ and treat $M$ as the sequence dimension. Then we directly put it into the spatial transformer encoder. 

During the decoding process, we repeat the reconstructed embedding $z_r$ with shape $[B, M, H]$ along with the temporal dimension to shape $[B, M, T, H]$. Then we follow the same process as the encoding process for spatial temporal decoding with a positional embedding added before the temporal transformer encoder.

\subsection{Details of metrics}
We provide details about the metrics we use in the experiment section.

\textbf{Maximum Mean Discrepancy (MMD)} is a statistical measure used to test the similarity of two distributions, denoted as $P$ and $Q$, by calculating the distance between the means of these distributions in a feature space defined by a kernel function. In our implementation, we use a Gaussian kernel $k(x, y)$ (also known as Radial Basis Function kernel). Assume we have samples $X=\{x_1,x_2,...,x_m\}$ from distribution $P$ and $Y=\{y_1, y_2,...,y_n\}$ from distribution $Q$, we calculate the MMD statistic as:
\begin{equation}
\begin{split}
    &\text{MMD}^2(P,Q) = \\
    &\frac{\sum_{i,j}k(x_i, x_j)}{m^2} + \frac{\sum_{i,j}k(y_i, y_j)}{n^2} + \frac{2\sum_{i,j}k(x_i, y_j)}{mn},
\end{split}
\end{equation}
where $m$ and $n$ are the number of samples from $P$ and $Q$ respectively. A larger MMD value indicates a greater discrepancy between the two distributions.

\textbf{Mean Average Displacement Error (mADE)} is a metric commonly used in the field of trajectory prediction, which quantifies the accuracy of predicted trajectories by comparing them with the actual trajectories. Assume the predicted trajectory is $\hat\tau_i = \{\hat{p}^i_1, \hat{p}^i_2,...,\hat{p}^i_T\}$ and the ground truth trajectory is $\tau_i = \{{p}^i_1, {p}^i_2,...,{p}^i_T\}$ for agent $i$ with trajectory length $T$, we calculate mADE with
\begin{equation}
    \text{mADE} = \frac{1}{N}\sum_{i=1}^N \left(\frac{1}{T}\sum_{t=1}^T \|\hat{p}^i_{t} - p^i_{t} \| \right),
\end{equation}
where $N$ is the number of agents in the validation dataset.

\textbf{Mean Final Displacement Error (mFDE)} is another important metric used in trajectory prediction, similar to mADE, but with a specific focus on the prediction accuracy at the final time step of the trajectories. With the same notation defined above, we calculate mFDE with 
\begin{equation}
    \text{mFDE} = \frac{1}{N}\sum_{i=1}^N \|\hat{p}^i_{T} - p^i_{T} \|.
\end{equation}

\textbf{Scene Collision Rate} is used to calculate the overlap between two vehicles for every timesteps in every trajectories. Specifically, a collision is said to occur between two vehicles if the Intersection Over Union (IOU) of their representing rectangles exceeds the threshold $\theta$:
\begin{equation}
    \text{Collision}(R_1, R_2) = 
\left\{
    \begin{array}{l}
        1, \text{if IOU}(R_1, R_2) > \theta \\
        0, \text{otherwise}
    \end{array}
\right.
\end{equation}
where the threshold $\theta$ is set to 0.1 and IOU is defined as:
\begin{equation}
    \text{IOU}(R_1, R_2) = \frac{\text{Area of Intersection ($R_1$, $R_2$)}}{\text{Area of Union ($R_1$, $R_2$)}}.
\end{equation}
Therefore, the scene collision rate is defined as:
\begin{equation}
    \text{Scene Collision Rate} = \frac{1}{N} \sum_{i=1}^N \text{Collision}(R_1, R_2).
\end{equation}

\textbf{Off-Road Rate} is used to calculate whether the trajectory is in the drivable area. We first calculate the indicator function of off-road with
\begin{equation}
    \text{Off-Road}(\tau_t) = 
\left\{
    \begin{array}{l}
        1, \text{if}\ \tau_t\ \text{not in drivable area} \\
        0, \text{otherwise}.
    \end{array}
\right.
\end{equation}
Then we calculate the rate with
\begin{equation}
    \text{Off-Road Rate} = \frac{1}{N}\sum_{i=1}^N \left(\frac{1}{T}\sum_{t=1}^T \text{Off-Road}(\tau_t^i) \right).
\end{equation}

\subsection{Hyper-parameters}

We list all important hyper-parameters we used during the training of the autonecoder and the combiner and the generation process in Table~\ref{tab:hyper_parameters}.

\subsection{Computational resources}

For all experiments, we use a server with AMD EPYC 7763 64-Core CPU, 256GB memory, and 4$\times$RTX A6000. 
The training of the autoencoder consumes 7.5GB memory and requires 8 hours on 1$\times$RTX A6000.
The training of the combiner consumes 2.1GB memory and requires 3 hours on 1$\times$RTX A6000.

\begin{table}[t]
\caption{Hyper-parameters}
\label{tab:hyper_parameters}
\centering
\scriptsize{
\begin{tabular}{c|c|c}
    \toprule
    Parameter Name                      &  Parameter Notation & Parameter Value \\
    \midrule 
    Max timestep                        & $T$         & 17 \\
    Max agent number                    & $M$         & 11 \\
    Trajectory frequency                &             & 2Hz \\
    Trajectory dimension meaning        &             & [x, y, v, cos(h), sin(h)] \\
    Map dimension meaning               &             & [x, y, cos(h), sin(h)] \\
    KNN Retrieve number                 & $K$         & 5 \\
    \midrule  
    Number of epochs (Autoencoder)      &             & 300 \\
    Batch size (Autoencoder)            &             & 64 \\
    Initial learning rate (Autoencoder) &     & 0.0008 \\
    Learning rate scheduler (Autoencoder)&             & MultiStepLR\\
    Scheduler parameter (Autoencoder)   &             & [20, 40, 60, 80, 100, 200]  \\
    Gradient clip                       &             & 5.0 \\
    Weight of InfoNCE loss              & $\lambda$   & 0.1 \\
    Temperature of InfoNCE              & $\tau$      & 0.1 \\
    Moments of Wasserstein distance     & $p$         & 2 \\
    Blur of Wasserstein distance        &             & 0.05 \\
    \midrule  
    Number of epochs (Combiner)         &             & 500 \\
    Batch size (Combiner)               &             & 64 \\
    Initial learning rate (Combiner)    &             & 0.001 \\
    Learning rate scheduler (Combiner)&             & MultiStepLR\\
    Scheduler parameter (Combiner)   &             & [20, 40, 60, 80, 100, 200]  \\
    \midrule  
    Radius for searching lanes          &             & 100 m \\
    Number of points in lane            &             & 20 \\
    Max number of lane                  &             & 100 \\
    Threshold for filtering static agent&             & 3 m \\
    \midrule
    Latent embedding dimension          & dim($z_b$), dim($z_i$), dim($z_m$) & 256 \\
    number of attention head            &             & 16 \\
    transformer feedforward dimension   &             & 512 \\
    dropout rate                        &             & 0.1 \\
    \midrule
    \# Behavior encoder layer           &  $L_e$      & 2 \\
    \# Behavior Spatial TransEnc layer  &             & 2 \\
    \# Behavior Temporal TransEnc layer &             & 1 \\
    Behavior projection MLP             &             & [5, 512] \\
    Initial pose projection MLP         &             & [5, 512] \\
    Map projection MLP                  &             & [4, 512] \\
    Map encoding MLP                    &             & [512, ReLU, Dropout, 512] \\
    \midrule
    \# Decoder layer number             &  $L_d$      & 2 \\
    \# Decoder Spatial TransEnc layer   &             & 2 \\
    \# Decoder Temporal TransEnc layer  &             & 1 \\
    Decoder projection MLP              &             & [512, ReLU, 512, ReLU, 5] \\
    \bottomrule
\end{tabular}
}
\end{table}

\section{More Experiment Results}
\label{sec:more_results}

We provide more experiment results in this section to demonstrate the performance of our method.

\begin{figure*}[t]
    \vspace{-3mm}
    \centering
    \includegraphics[width=1.0\textwidth]{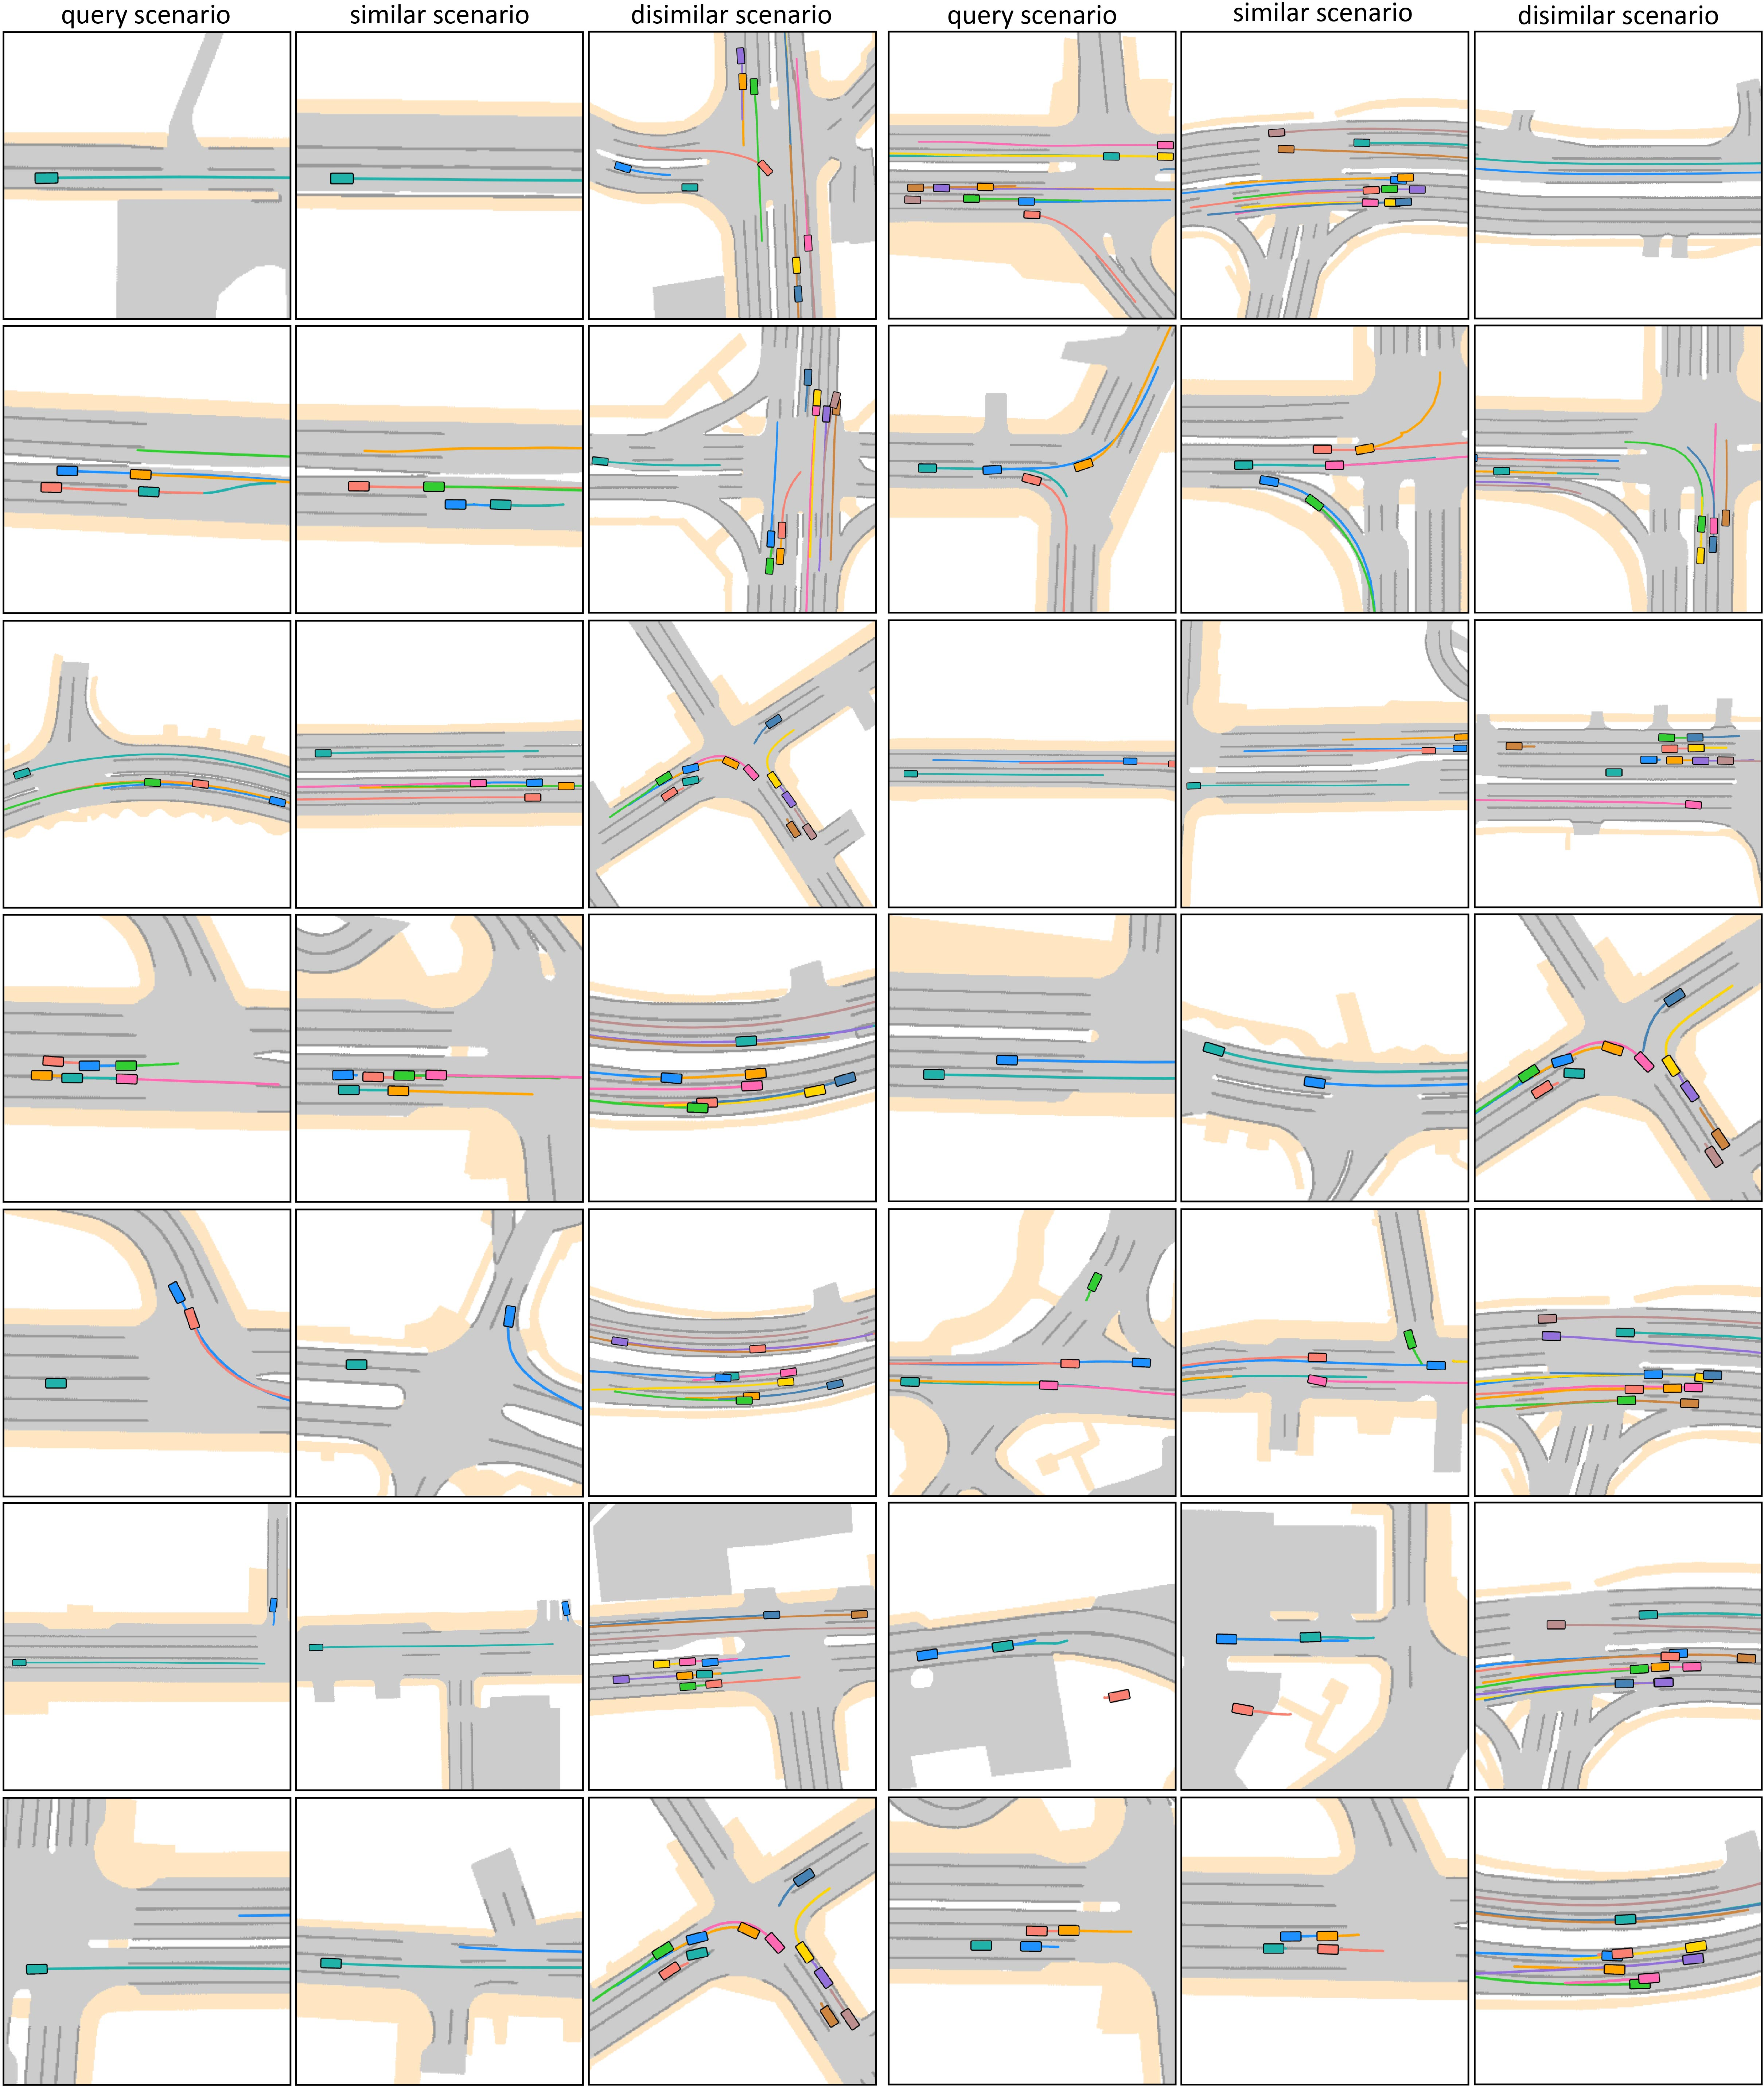}
    \vspace{-5mm}
    \caption{More examples of qualitative evaluation of similar and dissimilar scenarios calculated by our scenario embedding.}
    \label{fig:similar_scene_all}
    \vspace{-3mm}
\end{figure*}

\subsection{Visualization of failure cases}

In our experiments, we observe two types of failure cases for the retriever and generator, respectively.
As shown in Figure~\ref{fig:failure}(a), the retriever could fail because (1) the search database does not contain samples that are close to the complex query sample; (2) the number of vehicles rather than the interaction between vehicles influences the similarity a lot.
As shown in Figure~\ref{fig:failure}(b), the generator could fail mainly because the given initial pose and map do not match the retrieved behavior. For example, vehicles can not turn left when the initial positions are not near an intersection.

\begin{figure}[t]
    \centering
    \includegraphics[width=0.85\textwidth]{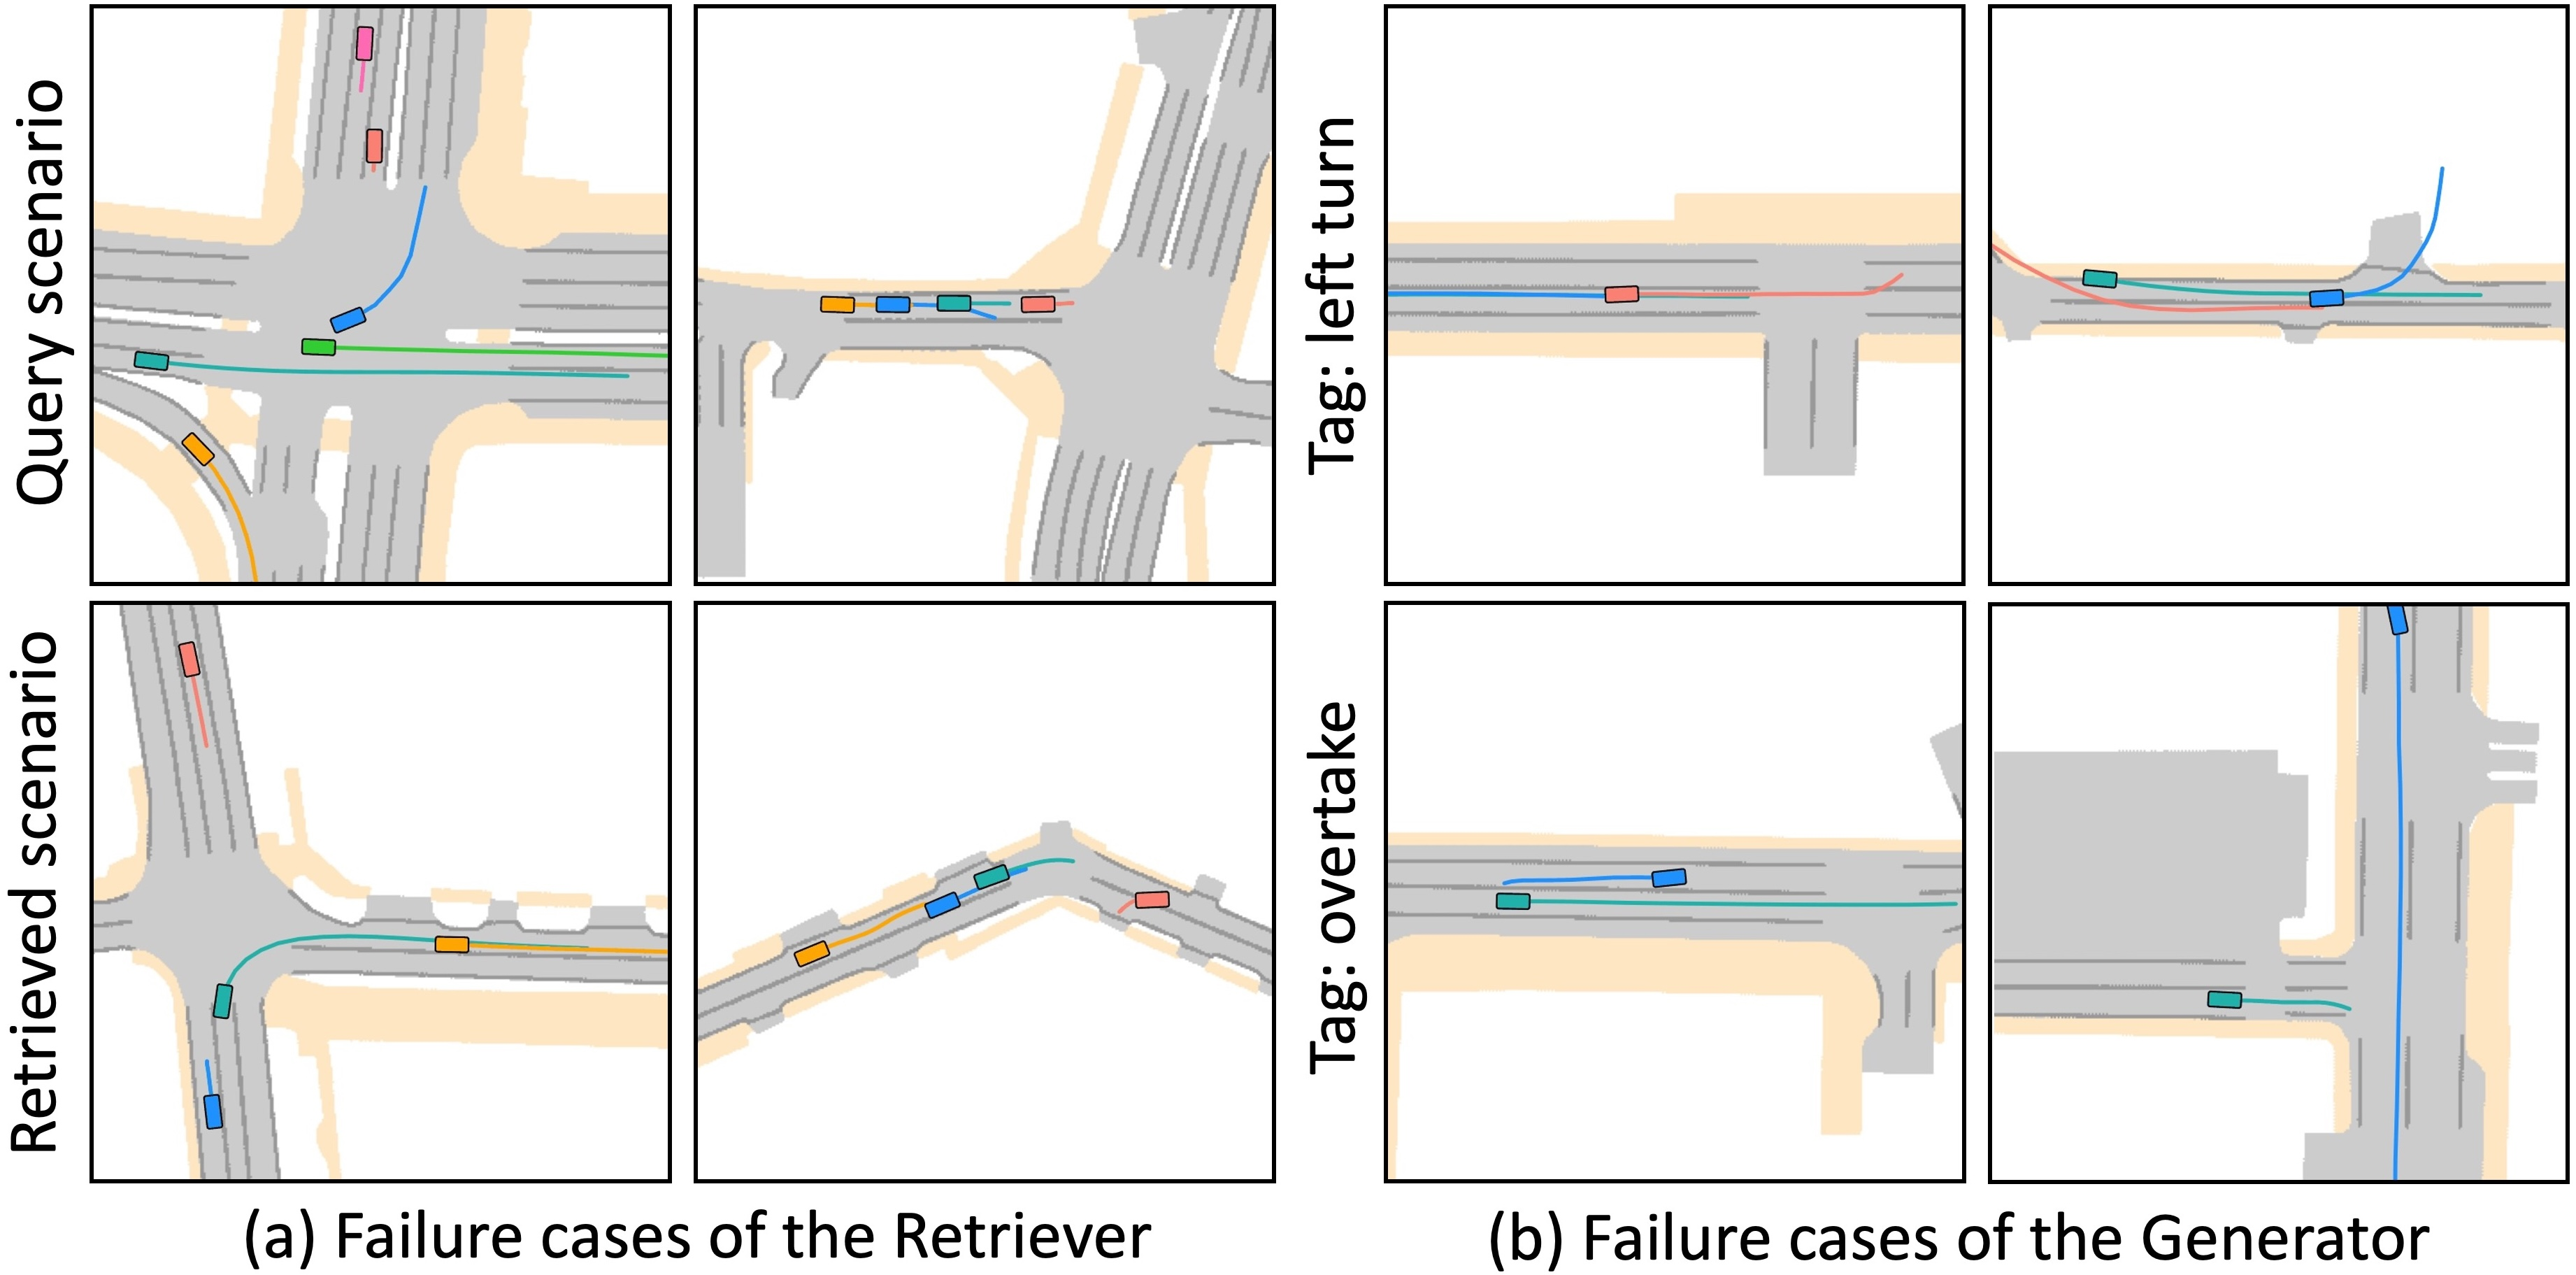}
    \vspace{-2mm}
    \caption{Failure case analysis.}
    \label{fig:failure}
    \vspace{-2mm}
\end{figure}

\subsection{Visualization of more retrieval results}

In Figure~\ref{fig:similar_scene_all}, we show more examples of scenarios similar and different from the query scenario.

\subsection{Visualization of feature invariance.} 
To demonstrate the invariance of the moving direction, we show the rotated input and reconstructed trajectories in Figure~\ref{fig:invariance}. We also calculate the distance between two scenarios, where one is rotated randomly from the other. Both results show that our auto-encoder model maps scenarios with different directions into very similar latent codes. 

\begin{figure}[t]
    \centering
    \includegraphics[width=0.9\textwidth]{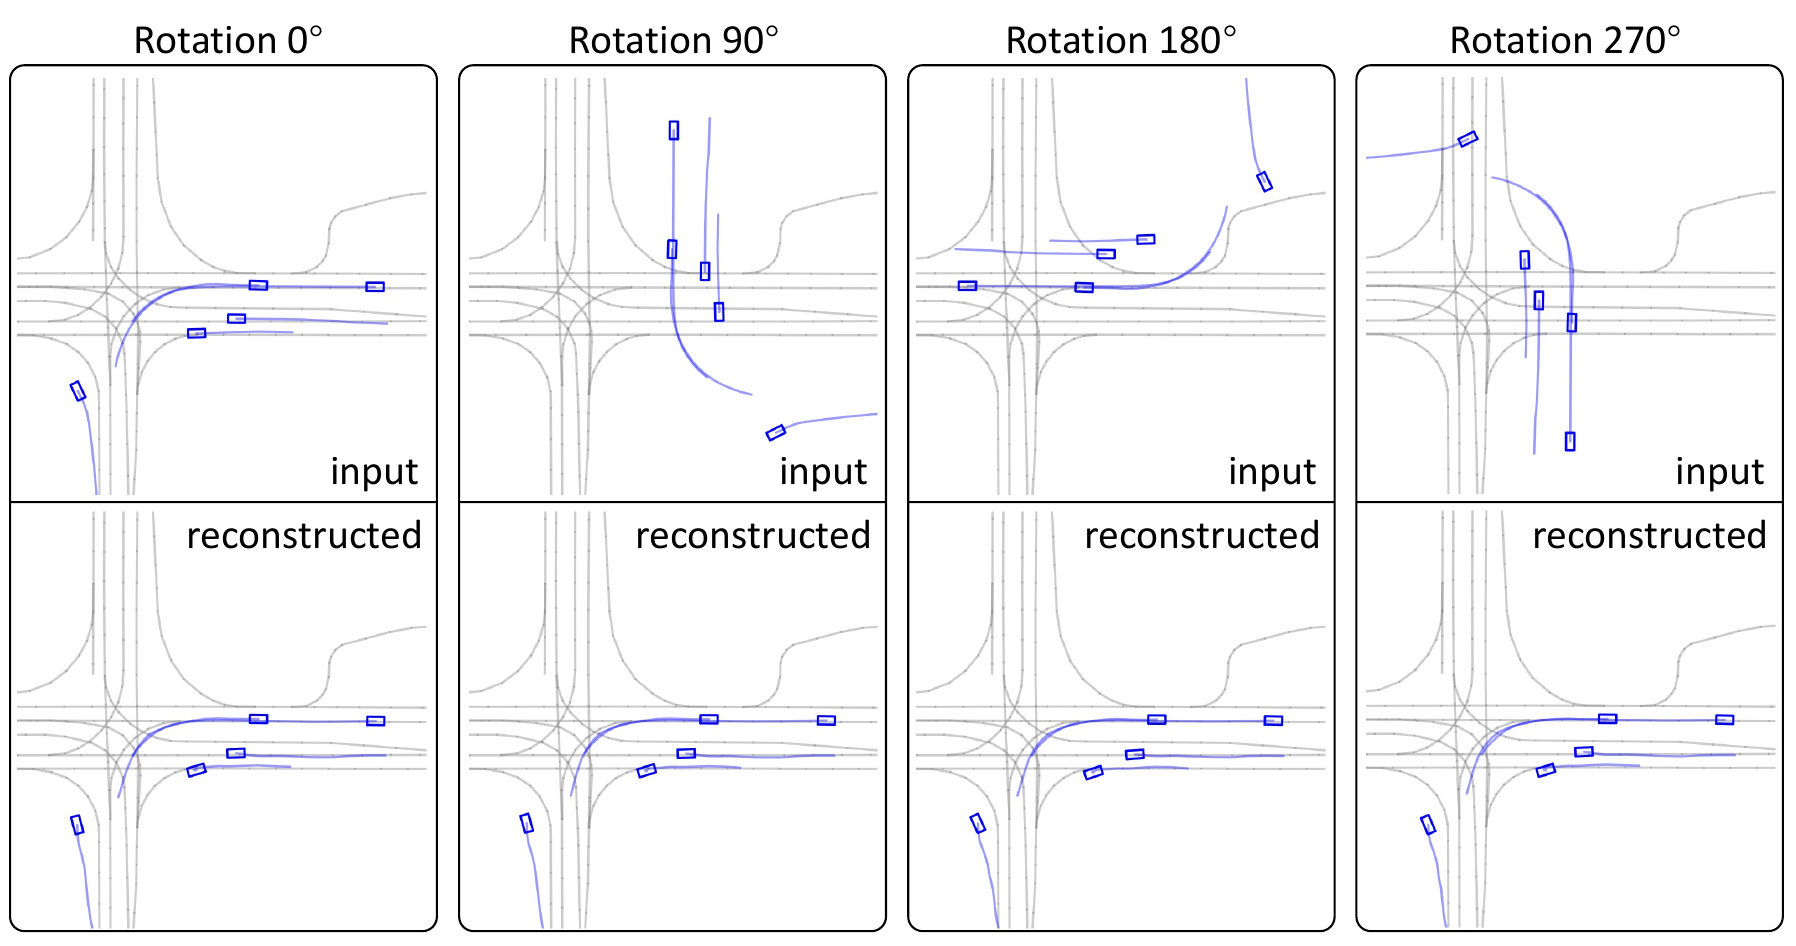}
    \caption{Reconstructions with rotated input trajectories.}
    \label{fig:invariance}
\end{figure}

\begin{table}[t]
\caption{Results of invariance evaluation.}
\label{tab:downstream}
\centering
\footnotesize{
\begin{tabular}{l|c|c|c|c|c|c}
    \toprule
    Degree       & 45$^\circ$ & 90$^\circ$ & 135$^\circ$ & 180$^\circ$ & 225$^\circ$ & 270$^\circ$ \\
    \midrule 
    Distance     & 0.001      & 0.004      & 0.006       & 0.008       & 0.006       & 0.004 \\
    \bottomrule
\end{tabular}
}
\end{table}

\subsection{Details of human evaluation}
\label{app:human}

For each category of scenarios, we select 10 examples from each generation algorithm. Each time, we ask a human evaluator to select one image from two images generated from our method and the baseline. The evaluator should also give a score (0-5) for both images. The final result is obtained by averaging the feedback from five evaluators. In Figure~\ref{fig:ab_testing}, we show some examples of the scenarios we used for the human evaluation.

\begin{figure*}[t]
    \vspace{-3mm}
    \centering
    \includegraphics[width=1.0\textwidth]{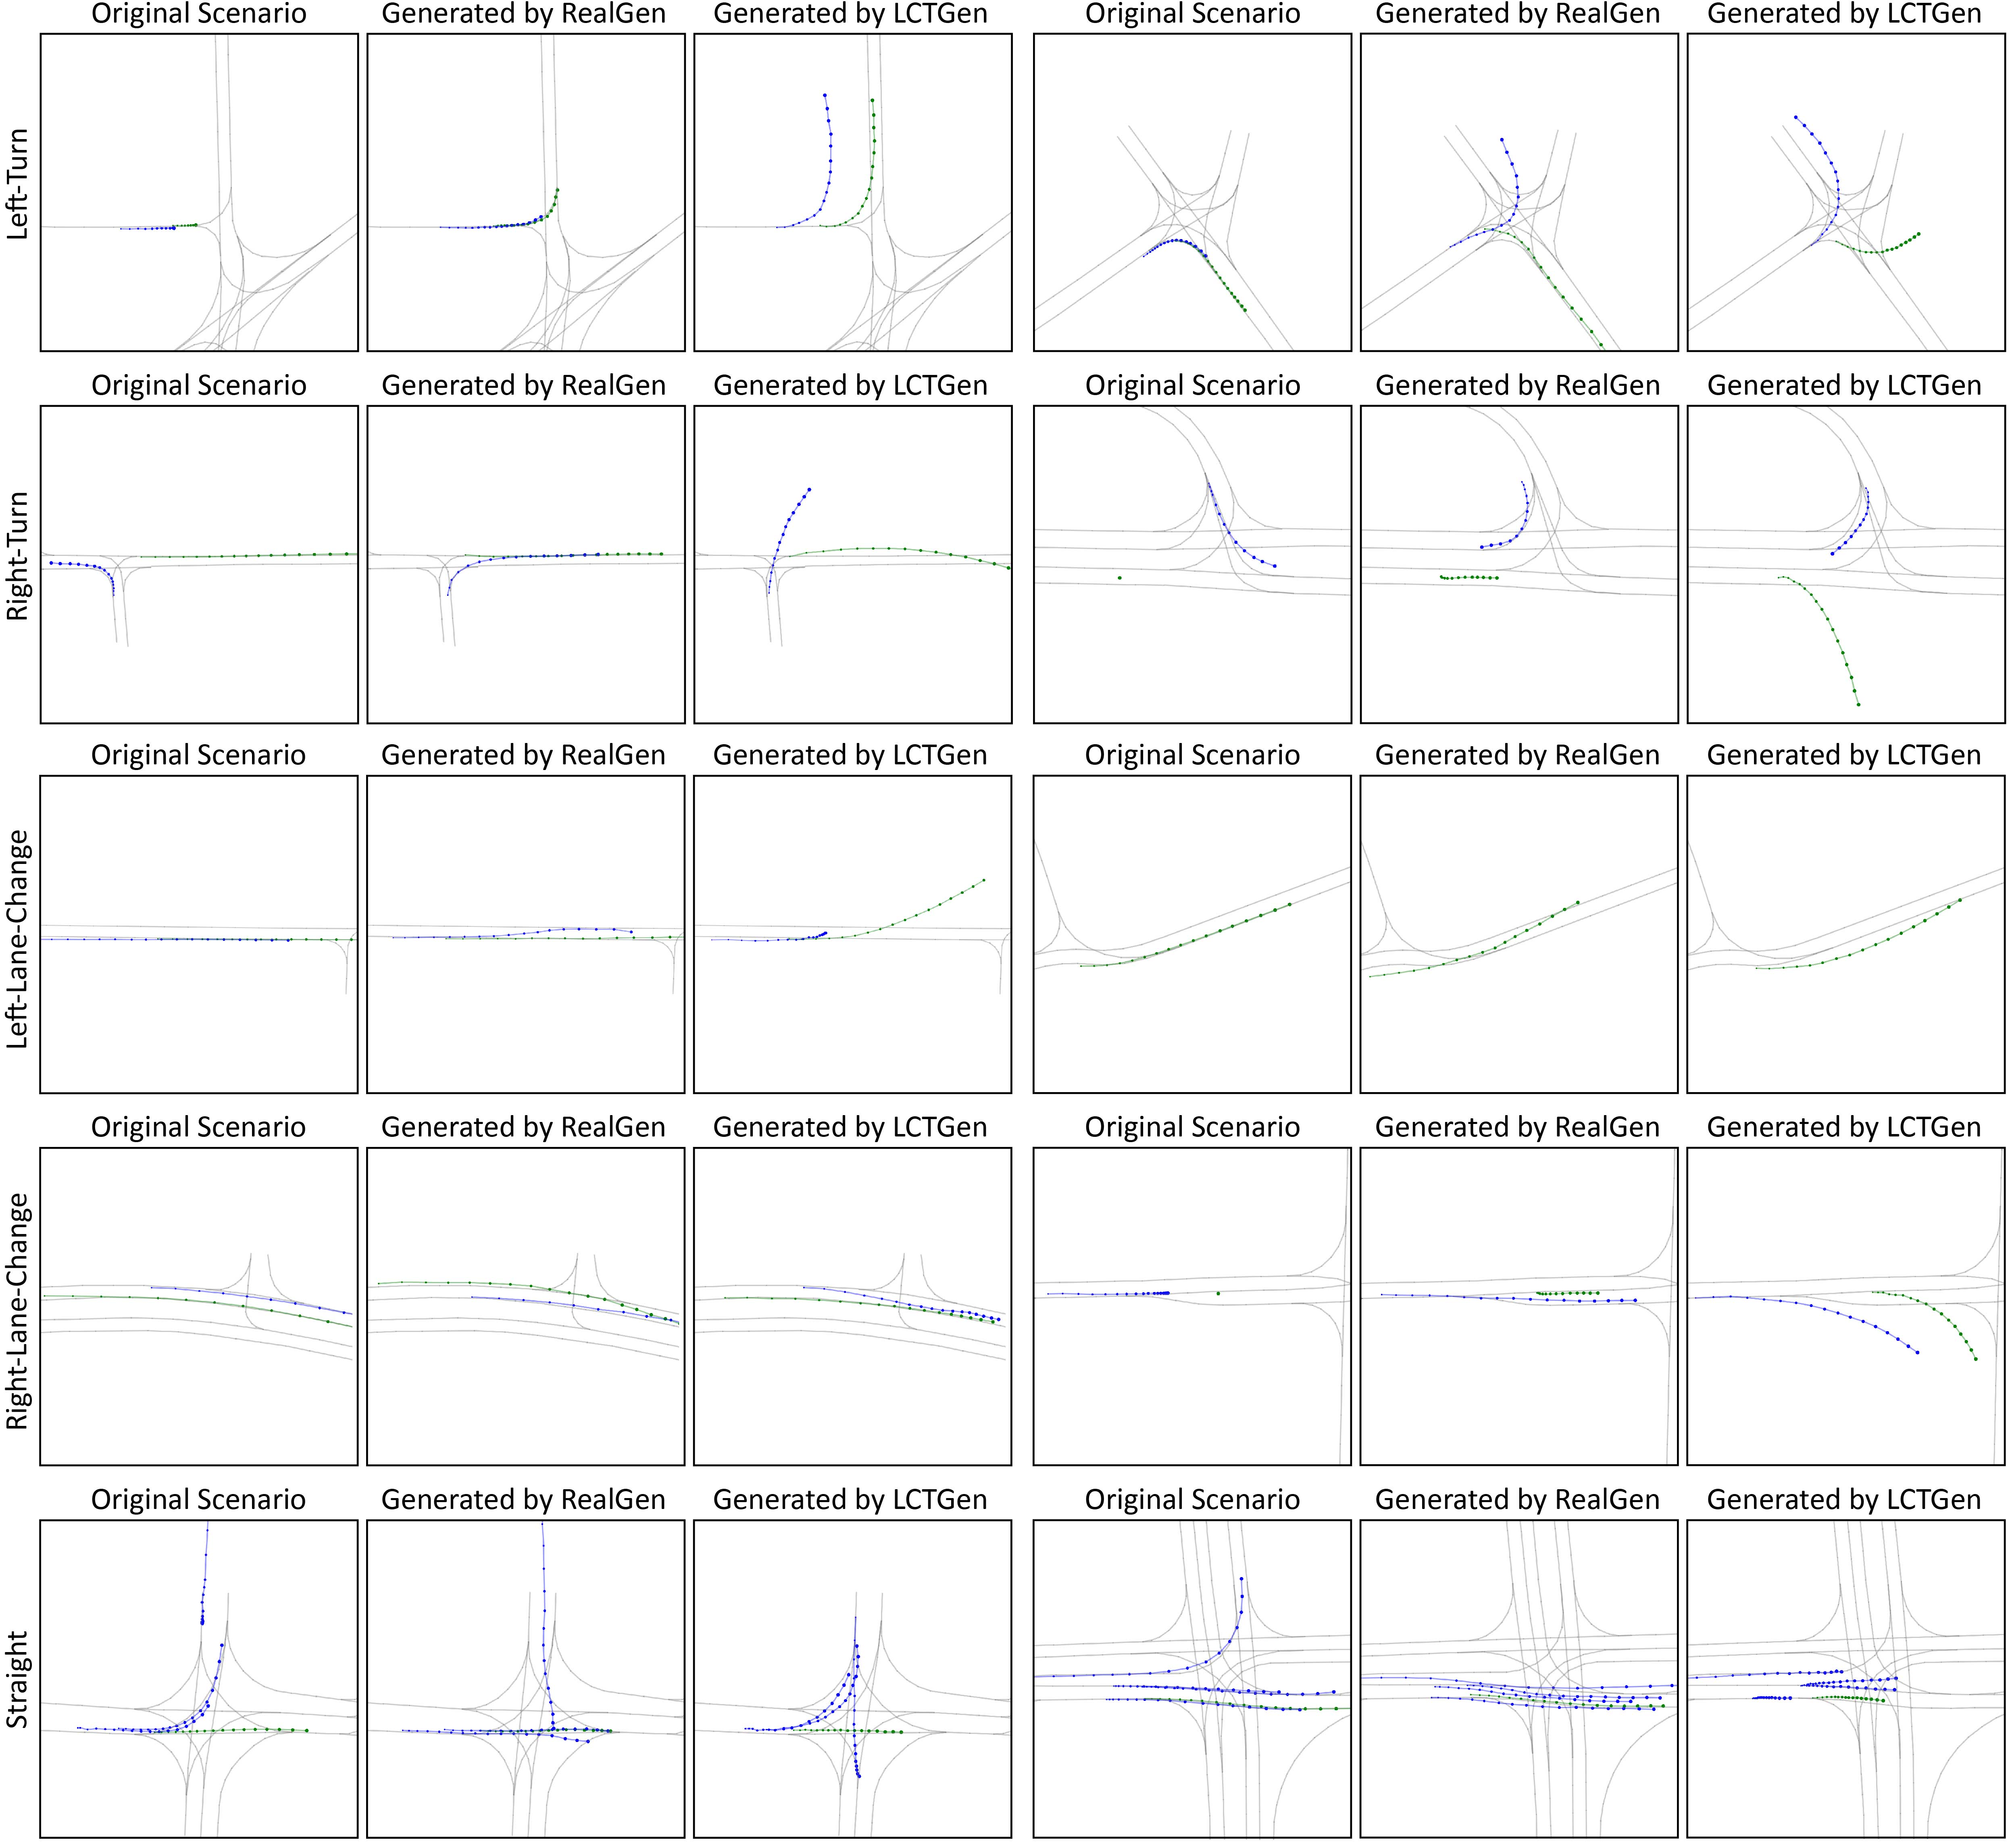}
    \vspace{-5mm}
    \caption{Examples of the scenarios we used for human evaluation of controllability. We used the map and initial positions of the original image (from nuScenes) to generate new scenarios using RealGen and LCTGen. We tested five scenario tags.}
    \label{fig:ab_testing}
    \vspace{-3mm}
\end{figure*}
